# Supplementary material for: The magnetic obliquity of accreting T Tauri stars
Source: arXiv:2007.06642 source file (2020-07-13)
Supplement: Supplementary file 1 [file onlinematerial_final.pdf]

# Online supplementary material for:
# The magnetic obliquity of accreting T Tauri stars

Pauline McGinnis[1,2], Jérôme Bouvier[2] and Florian Gallet[2]
[1]Dublin Institute for Advanced Studies, A&A Section, 31 Fitzwilliam Place, Dublin 2, D02 XF86, Ireland
[2]Univ. Grenoble Alpes, CNRS, IPAG, F-38000 Grenoble, France
Corresponding author: pmcginnis@cp.dias.ie

## Appendix C: CCF profiles

Figure S1 shows the cross-correlation functions (CCF) obtained for the 12 T Tauri stars investigated in this paper. Some stars display deep and symmetric CCF profiles, which exhibit limited night-to-night variations that can probably be accounted for by spot modulation. This is the case for, e.g., DN Tau, DE Tau, GI Tau, GM Aur, IW Tau, and V836 Tau. To our knowledge, V826 Tau is the only previously reported SB2 in this sample (Mundt et al. 1983), which we easily confirm from its rapidly varying, double-dip CCF profile (partially truncated over the CCF velocity range computed here). Large night-to-night CCF variations are observed for the other objects: DF Tau (but the signal-to-noise is low and the CCF is shallow), DK Tau, GK Tau, IP Tau, and T Tau. Their large CCF variations are reflected in the radial velocity scatter, $\sigma V_{rad}$, listed in Table 1 of the paper. IP Tau has a relatively narrow CCF and its variations might result from large spots at the stellar surface. In contrast, DK Tau, GK Tau, and T Tau exhibit a wide CCF with considerable structure and shape variations. On one occurrence (Nov.23, UT 21:28), GK Tau displays a clear double-dip CCF profile, reminiscent of a SB2. Whether the spectacular CCF night-to-night variations seen in these 3 objects are due to surface spots, circumstellar environment, or binarity is unclear.

## Appendix D: Normalized spectra

Figure S2 shows the normalized spectra of the T Tauri stars in our sample in the range from 5850Å to 5900Å. The night to night variability of the He I line, and in a few cases of the veiling (observed by the change in depth of photospheric absorption lines), can be seen. The Na I doublet at 5890Å and 5896Å can also be verified on the right-hand side of these plots.

## Appendix E: Gaussian decomposition of the star T Tau

Figure S3 shows the Gaussian decomposition of the He I line profile for each individual observation of the star T Tau. Two observations were excluded from Fig. 5 of the main paper due to their low S/N and therefore are not shown here.

## Appendix F: LiI$\lambda$6708, H$\alpha$ and H$\beta$ line profiles

The LiI$\lambda$6708 line profiles for our stellar sample are shown in Fig. S4. Most of the sources display quite symmetric line profiles, with the noticeable exception of V826 Tau, an SB2 system. The Li I line depth hardly varies for most sources (DN Tau, DF Tau, DE Tau, IW Tau, T Tau, V836 Tau), which indicates little veiling variations occurred over the course of our observations. Nevertheless, significant intensity variations are seen in the Li I line core of DK Tau, GK Tau, and IP Tau, as well as small intensity variations in that of GI Tau and GM Aur. In these five cases the Li I line equivalent width is inversely correlated with the strength of the HeI$\lambda$5876 line. Such a behaviour is expected from a rotating hotspot resulting from a localized accretion shock at the stellar surface. At maximum visibility, the He I line formed in the accretion shock reaches its highest intensity while the Li I line becomes shallower due to enhanced continuum emission from the shock (veiling).

The H$\alpha$ and H$\beta$ line profiles that were discussed in the text are shown in Figs. S5 and S6 superimposed onto each other, in order to highlight their night-to-night variability.

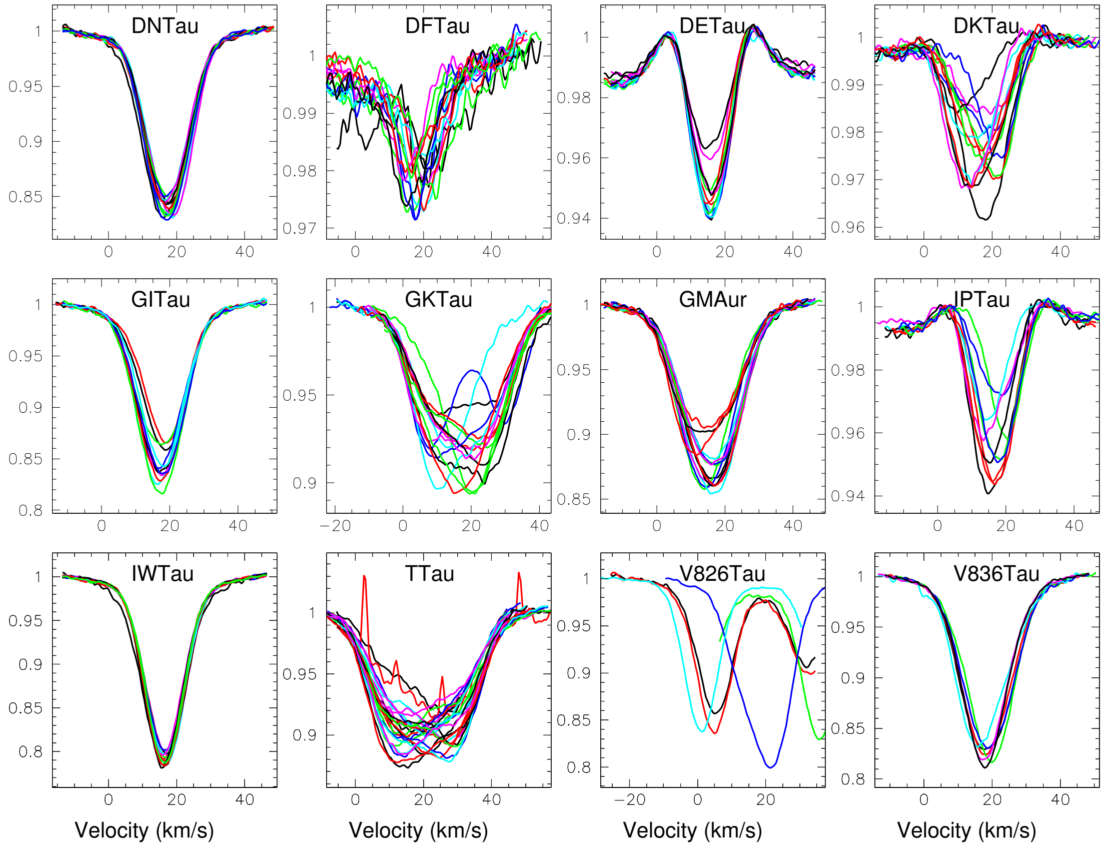


Figure S1: Night-to-night cross-correlation (CCF) profiles are shown for the sample of 12 T Tauri stars investigated here, shown superimposed on each other to highlight their variability. CCF profiles have been normalized at the 90 percentile flux level. We note that V826 Tau is a known SB2.

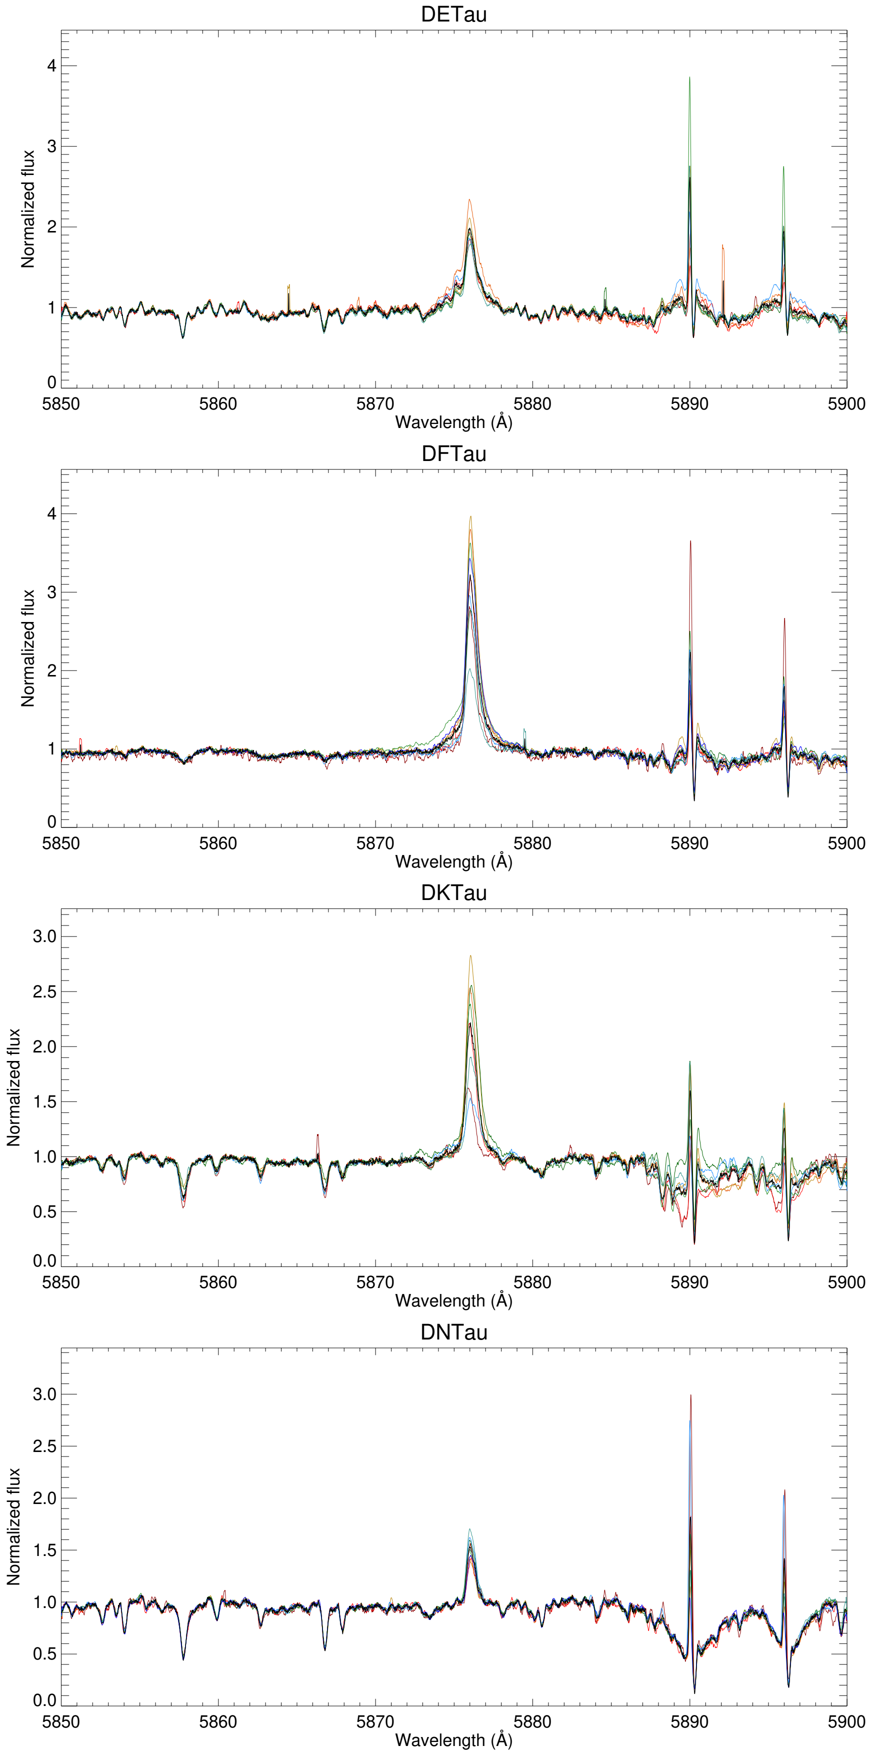


Figure S2: Normalized spectra around the HeI$\lambda$5876 line for all stars in our sample. Colored lines represent spectra of individual nights, while the bold black line shows the average spectrum.

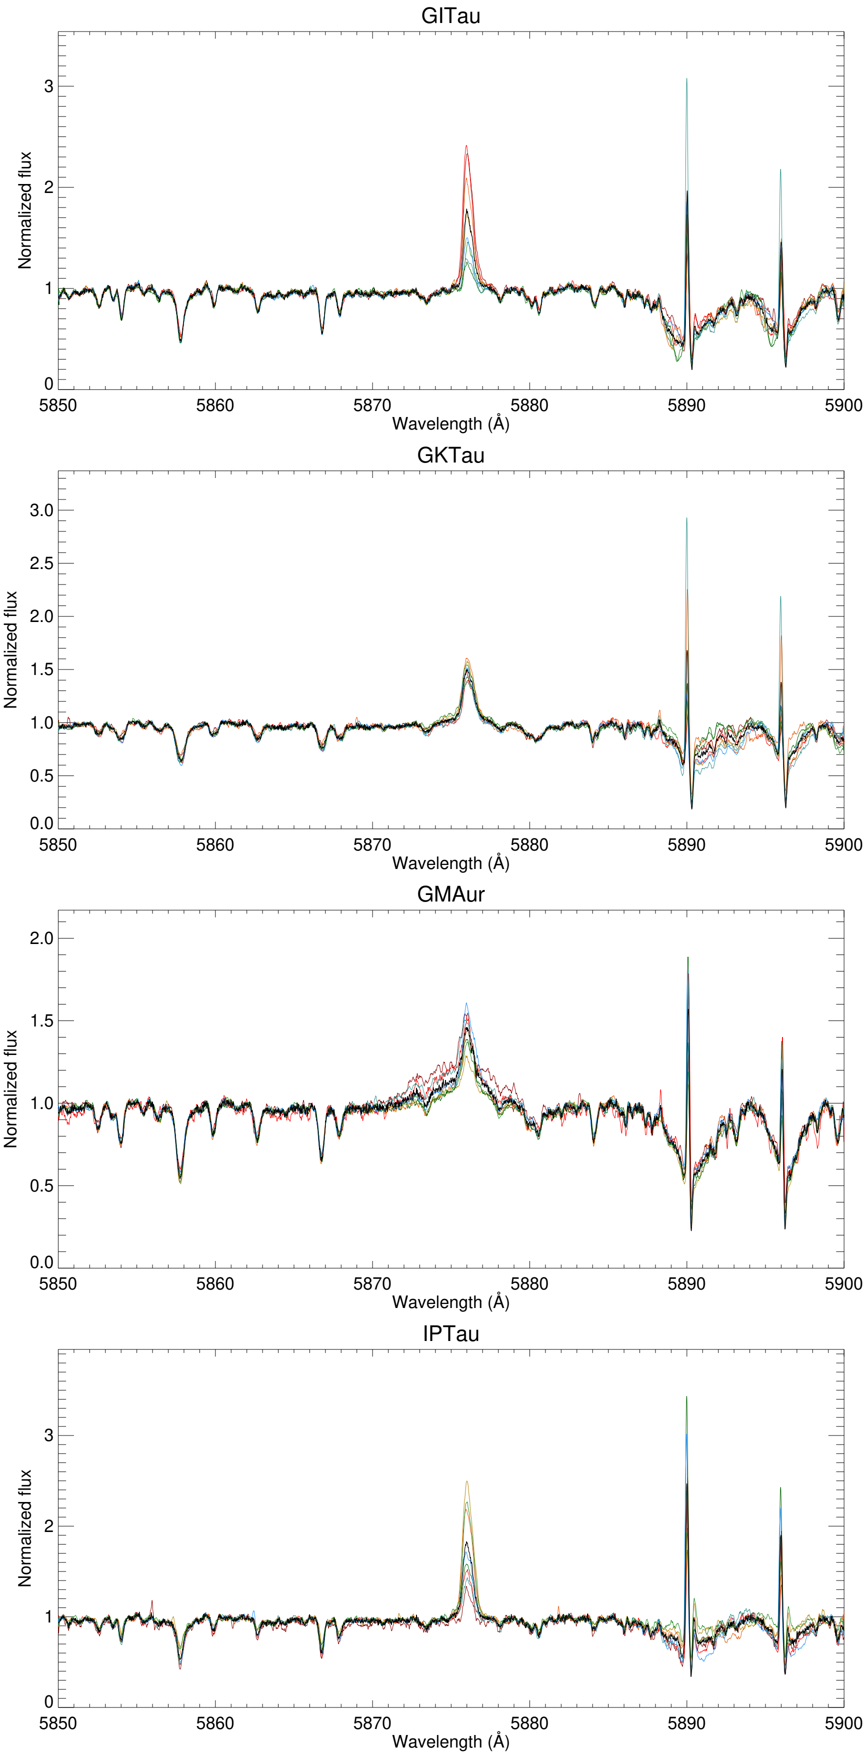


Figure S2: Continued.

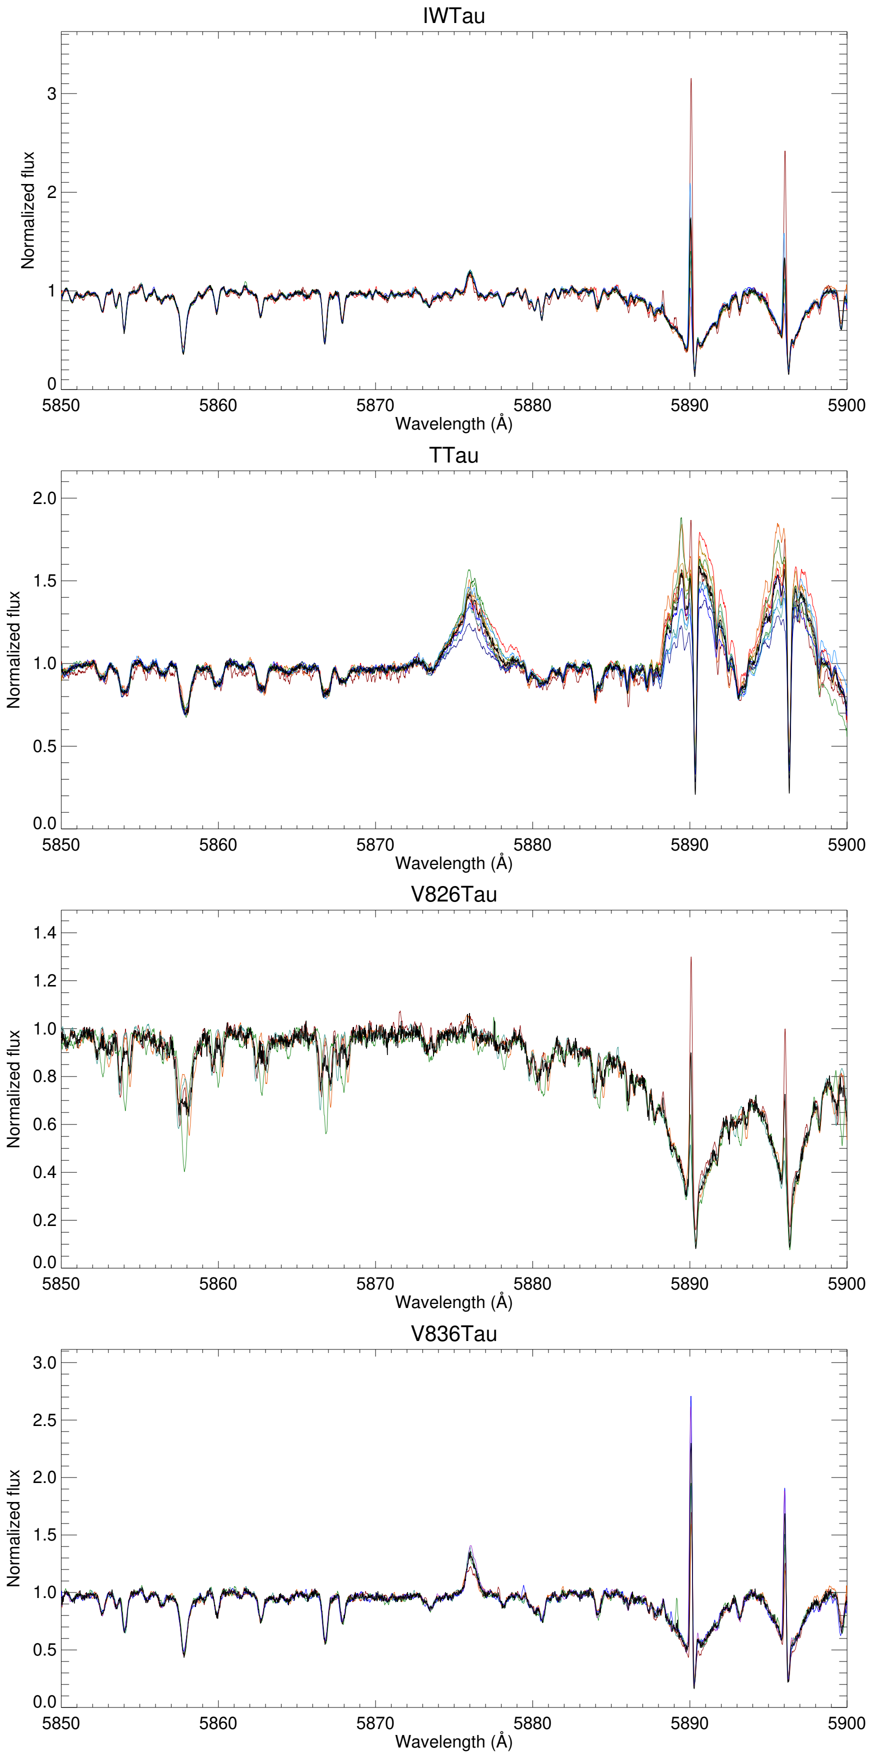


Figure S2: Continued.

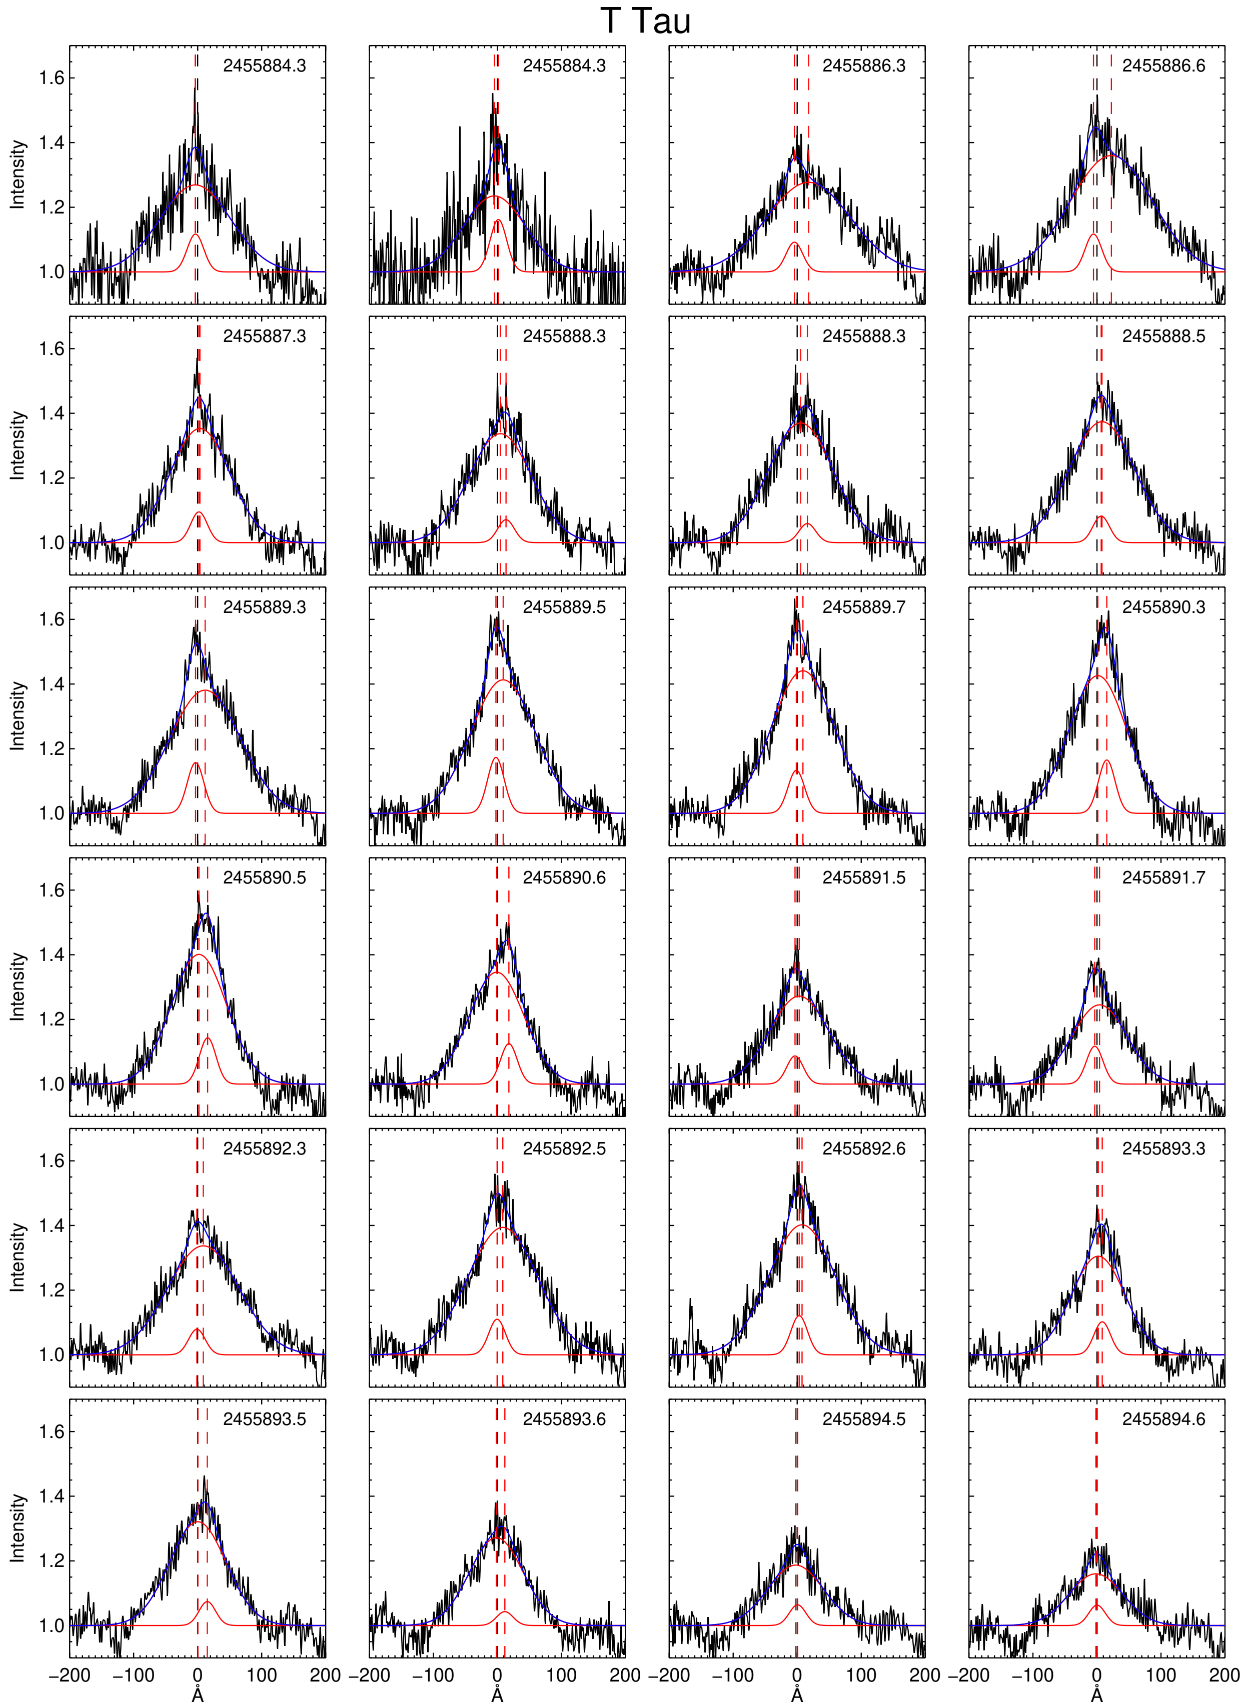


Figure S3: Gaussian decomposition of the He I line profile for each individual observation of the star T Tau. Black lines show the observed profiles, red lines represent the two Gaussian components used in the fit and blue lines represent the sum of the two components. The black dashed lines give the line center at stellar rest velocity while the red dashed lines show the centroid velocity of the two Gaussian components. Julian dates for each observation are given at the top right of each plot.

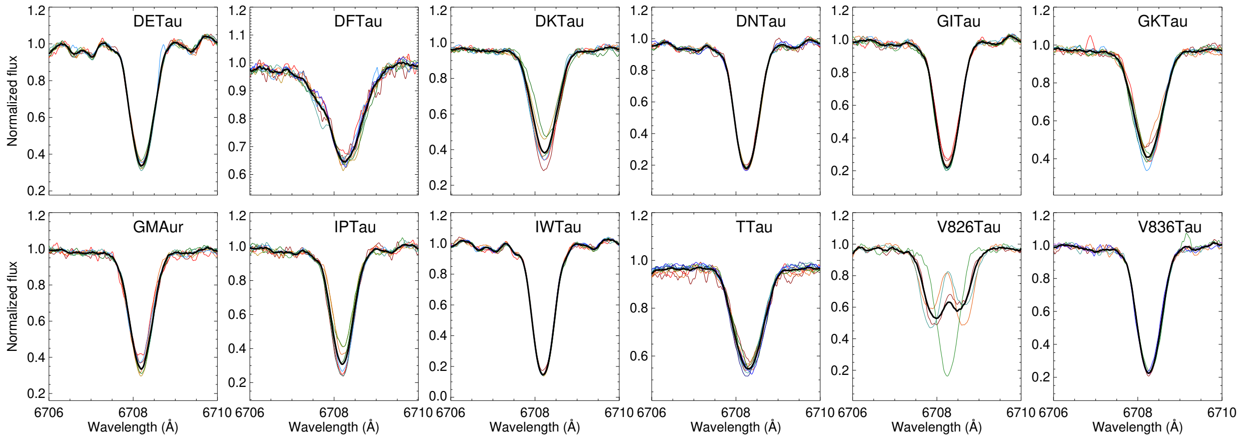


Figure S4: The LiI$\lambda$6708 line profile of CTTS and WTTS observed in this study. *Thin lines:* individual line profiles. *Thick black line:* averaged Li I line profile. For clarity, the profiles shown here have been boxcar smoothed over 15 pixels (0.15 Å).

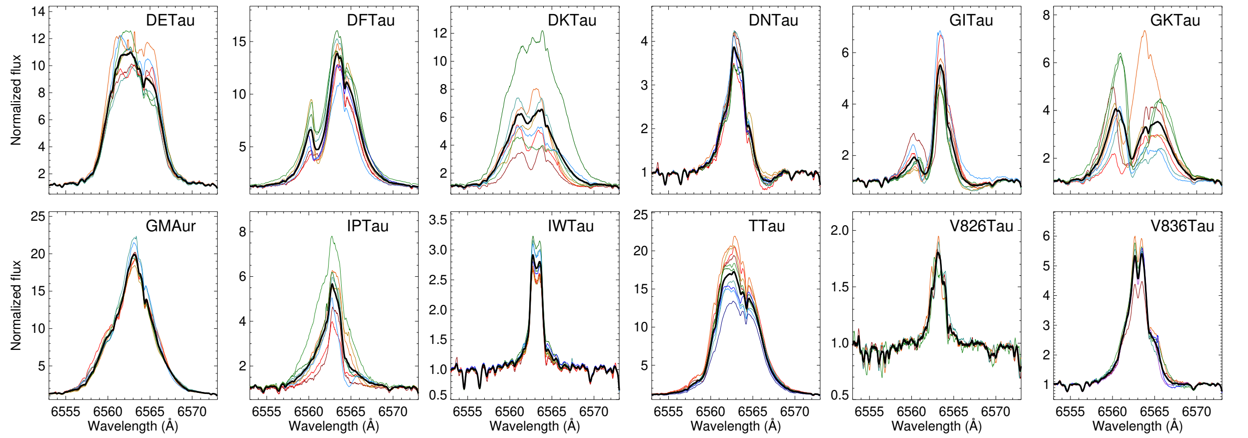


Figure S5: The H$\alpha$ line profile of CTTS and WTTS observed in this study. Lines and smoothing are the same as in the previous figure.

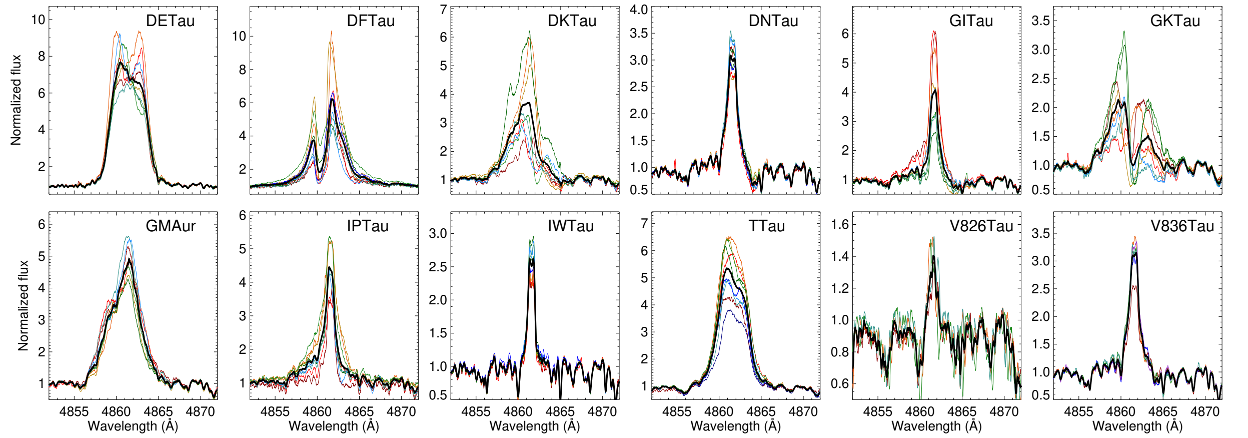


Figure S6: The H$\beta$ line profile of CTTS and WTTS observed in this study. Lines and smoothing are the same as in the previous figure.
